# Supplementary material for: An infinite family of 2-groups with mixed Beauville structures
Source: arXiv:1304.4480 ancillary file (2013-04-16)
Supplement: Supplementary file 1 [file procedures.pdf]

# MAPLE PROCEDURES FOR "AN INFINITE FAMILY OF 2-GROUPS WITH MIXED BEAUVILLE STRUCTURES"

NATHAN BARKER, NIGEL BOSTON, NORBERT PEYERIMHOFF,  
AND ALINA VDOVINA

## 1. USEFUL TRANSFORMATION PROCEDURES

The following procedure transforms a number  $0 \leq n \leq 511$  into a  $3 \times 3$  matrix  $u$ :

```
transfnm := proc(n)
local m1, m2, u11, u12, u13, u21, u22, u23, u31, u32, u33, u;
m1 := n;
u11 := iquo(m1, 256); m2 := irem(m1, 256);
u12 := iquo(m2, 128); m1 := irem(m2, 128);
u13 := iquo(m1, 64); m2 := irem(m1, 64);
u21 := iquo(m2, 32); m1 := irem(m2, 32);
u22 := iquo(m1, 16); m2 := irem(m1, 16);
u23 := iquo(m2, 8); m1 := irem(m2, 8);
u31 := iquo(m1, 4); m2 := irem(m1, 4);
u32 := iquo(m2, 2);
u33 := irem(m2, 2);
u := Matrix([[u11, u12, u13], [u21, u22, u23], [u31, u32, u33]])
end proc
```

The following procedure transforms a  $3 \times 3$  matrix  $u$  into a number  $0 \leq n \leq 511$ :

```
transfmn := proc(u)
local n;
n := 256*u[1,1]+128*u[1,2]+64*u[1,3]+32*u[2,1]+16*u[2,2]+8*u[2,3]
+4*u[3,1]+2*u[3,2]+u[3,3];
end proc
```

The following procedure extracts from a  $3 \times 9$ -matrix  $U$  the  $k$ -th  $3 \times 3$ -matrix  $uk$ , where  $1 \leq k \leq 3$ :

```
extract := proc(k,U)
local uk;
if k = 1 then uk := Matrix([[U[1,1], U[1,2], U[1,3]], [U[2,1],
U[2,2], U[2,3]], [U[3,1], U[3,2], U[3,3]]])
elif k = 2 then uk := Matrix([[U[1,4], U[1,5], U[1,6]], [U[2,4],
U[2,5], U[2,6]], [U[3,4], U[3,5], U[3,6]]])
else uk := Matrix([[U[1,7], U[1,8], U[1,9]], [U[2,7], U[2,8],
U[2,9]], [U[3,7], U[3,8], U[3,9]]])
end if;
uk
end proc
```

The following procedure combines three  $3 \times 3$ -matrices  $u_1, u_2, u_3$  into a  $3 \times 9$ -matrix  $U$ :

```
comb := proc(u1,u2,u3)
local U;
U := Matrix([[u1[1,1], u1[1,2], u1[1,3], u2[1,1], u2[1,2], u2[1,3],
u3[1,1], u3[1,2], u3[1,3]], [u1[2,1], u1[2,2], u1[2,3], u2[2,1],
u2[2,2], u2[2,3], u3[2,1], u3[2,2], u3[2,3]], [u1[3,1], u1[3,2],
u1[3,3], u2[3,1], u2[3,2], u2[3,3], u3[3,1], u3[3,2], u3[3,3]]])
end proc
```

The following procedure transforms a list  $[k, a_1, a_2]$  with  $k \geq 0$  and  $a_1, a_2 \in \{0, 1, \dots, 511\}^3$ , representing a matrix  $M_k(a_1, a_2, \dots)$ , into another list  $[k, U_1, U_2]$  where  $U_1, U_2$  are the  $3 \times 9$ -matrices corresponding to  $a_1$  and  $a_2$ :

```
transfinp := proc(z)
local k, a1, a2, a11, a12, a13, a21, a22, a23, U1, U2, u11,
u12, u13, u21, u22, u23;
k := op(1,z); a1 := op(2,z); a2 := op(3,z);
a11 := op(1,a1); a12 := op(2,a1); a13 := op(3,a1);
a21 := op(1,a2); a22 := op(2,a2); a23 := op(3,a2);
u11 := transfnm(a11); u12 := transfnm(a12); u13 := transfnm(a13);
u21 := transfnm(a21); u22 := transfnm(a22); u23 := transfnm(a23);
U1 := comb(u11, u12, u13); U2 := comb(u21, u22, u23);
[k, U1, U2]
end proc
```

The following procedure transforms a list  $[k, U_1, U_2]$  with  $k \geq 0$  and  $U_1, U_2$  two  $3 \times 9$ -matrices, representing a matrix  $M_k(U_1, U_2, \dots)$ , into another list  $zout = [k, a_1, a_2]$  where  $a_1, a_2$  are the triples in  $\{0, 1, \dots, 511\}^3$  corresponding to  $U_1$  and  $U_2$ :

```

outp := proc(z)
local k, U1, U2, zout;
k := op(1,z); U1 := op(2,z); U2 := op(3,z);
zout := [k, [transfmn(extract(1,U1)), transfmn(extract(2,U1)),
transfmn(extract(3,U1))], [transfmn(extract(1,U2)),
transfmn(extract(2,U2)), transfmn(extract(3,U2))]]
end proc

```

## 2. MATRIX OPERATIONS

The following procedure calculates for a given element  $[k, U_1, U_2]$ , representing a matrix  $M_k(U_1, U_2, \dots)$ , the square  $[2k + 1, V_1, V_2]$ , representing a matrix  $M_{2k+1}(V_1, V_2, \dots) = M_k(U_1, U_2, \dots)^2$ :

```

power2 := proc(z)
local k, U1, U2, u11, u12, u13, u21, u22, u23, zsq, V1, V2,
v11, v12, v13, v21, v22, v23;
k := op(1,z); U1 := op(2,z); U2 := op(3,z);
u11 := extract(1,U1); u12 := extract(2,U1); u13 := extract(3,U1);
u21 := extract(1,U2); u22 := extract(2,U2); u23 := extract(3,U2);
if modp(k,3) = 0 then
v11 := 'mod'(u11.u12,2); v12 := 'mod'(u12.u13,2);
v13 := 'mod'(u13.u11,2); v21 := 'mod'(u11.u22+u21.u13,2);
v22 := 'mod'(u12.u23+u22.u11,2); v23 := 'mod'(u13.u21+u23.u12,2)
elif modp(k,3) = 1 then
v11 := 'mod'(u11.u13,2); v12 := 'mod'(u12.u11,2);
v13 := 'mod'(u13.u12,2); v21 := 'mod'(u11.u23+u21.u11,2);
v22 := 'mod'(u12.u21+u22.u12,2); v23 := 'mod'(u13.u22+u23.u13,2)
else
v11 := 'mod'(u11.u11,2); v12 := 'mod'(u12.u12,2);
v13 := 'mod'(u13.u13,2); v21 := 'mod'(u11.u21+u21.u12,2);
v22 := 'mod'(u12.u22+u22.u13,2); v23 := 'mod'(u13.u23+u23.u11,2)
end if;
V1 := comb(v11,v12,v13); V2 := comb(v21,v22,v23);
zsq := [2*k+1,V1,V2]
end proc

```

The following procedure calculates for a given element  $[0, U_1, U_2]$ , representing a matrix  $M_0(U_1, U_2, \dots)$ , the inverse  $[0, V_1, V_2]$ , representing a matrix  $M_0(V_1, V_2, \dots) = M_0(U_1, U_2, \dots)^{-1}$ :

```

invers := proc(z)
local U1, U2, u11, u12, u13, u21, u22, u23, zinv, V1, V2, v21,
v22, v23;
U1 := op(2,z); U2 := op(3,z);
u11 := extract(1,U1); u12 := extract(2,U1); u13 := extract(3,U1);
u21 := extract(1,U2); u22 := extract(2,U2); u23 := extract(3,U2);
v21 := 'mod'(u11.u12+u21,2); v22 := 'mod'(u12.u13+u22,2);
v23 := 'mod'(u13.u11+u23,2);
V1 := U1; V2 := comb(v21,v22,v23);
zinv := [0,V1,V2]
end proc

```

The following procedure calculates for given elements  $[0, U_1, U_2]$  and  $[0, V_1, V_2]$ , representing matrices  $M_0(U_1, U_2, \dots)$  and  $M_0(V_1, V_2, \dots)$ , their product  $[0, W_1, W_2]$ , representing a matrix  $M_0(W_1, W_2, \dots) = M_0(U_1, U_2, \dots)M_0(V_1, V_2, \dots)$ :

```

prod := proc(z1,z2)
local U1, U2, u11, u12, u13, u21, u22, u23, V1, V2, v11, v12,
v13, v21, v22, v23, zout, W1, W2, w11, w12, w13, w21, w22, w23;
U1 := op(2,z1); U2 := op(3,z1);
u11 := extract(1,U1); u12 := extract(2,U1); u13 := extract(3,U1);
u21 := extract(1,U2); u22 := extract(2,U2); u23 := extract(3,U2);
V1 := op(2,z2); V2 := op(3,z2);
v11 := extract(1,V1); v12 := extract(2,V1); v13 := extract(3,V1);
v21 := extract(1,V2); v22 := extract(2,V2); v23 := extract(3,V2);
w11 := 'mod'(u11+v11,2); w12 := 'mod'(u12+v12,2);
w13 := 'mod'(u13+v13,2); w21 := 'mod'(u21+v21+u11.v12,2);
w22 := 'mod'(u22+v22+u12.v13,2); w23 := 'mod'(u23+v23+u13.v11,2);
W1 := comb(w11,w12,w13); W2 := comb(w21,w22,w23);
zout := [0, W1, W2]
end proc

```

The following procedure calculates for a given  $3 \times 9$ -matrix  $U$  and an element  $[k, V_1, V_2]$ , representing a matrix  $M_k(V_1, V_2, \dots)$ , the conjugate element  $[k, V_1, W_2]$ , representing a matrix  $M_k(V_1, W_2, \dots) = M_0(U, \dots)^{-1} M_k(V_1, V_2, \dots) M_0(U, \dots)$ :

```
conj := proc(U,z)
local u1, u2, u3, k, V1, V2, v11, v12, v13, v21, v22, v23, zconj,
W2, w11, w12, w13, w21, w22, w23;
k := op(1,z); V1 := op(2,z); V2 := op(3,z);
v11 := extract(1,V1); v12 := extract(2,V1); v13 := extract(3,V1);
v21 := extract(1,V2); v22 := extract(2,V2); v23 := extract(3,V2);
u1 := extract(1,U); u2 := extract(2,U); u3 := extract(3,U);
if modp(k,3) = 0 then w21 := 'mod'(v21+u1.v12+v11.u2,2);
w22 := 'mod'(v22+u2.v13+v12.u3,2); w23 := 'mod'(v23+u3.v11+v13.u1,2)
elif 'mod'(k,3) = 1 then w21 := 'mod'(v21+u1.v12+v11.u3,2);
w22 := 'mod'(v22+u2.v13+v12.u1,2); w23 := 'mod'(v23+u3.v11+v13.u2,2)
else w21 := 'mod'(v21+u1.v12+v11.u1,2);
w22 := 'mod'(v22+u2.v13+v12.u2,2); w23 := 'mod'(v23+u3.v11+v13.u3,2)
end if;
W2 := comb(w21,w22,w23);
zconj := [k,V1,W2]
end proc
```

### 3. USING THE ABOVE PROCEDURES FOR EXPLICIT CALCULATIONS

The following lines create the elements  $x_0, x_1, x, y_0, y_1, y$ :

```
x0 := transfinp([0, [11, 11, 11], [17, 17, 17]]):
x1 := transfinp([0, [23, 224, 138], [59, 136, 495]]):
x2 := transfinp([0, [46, 68, 217], [12, 194, 363]]):
x := prod(invers(x1), invers(x0)): x2inv := invers(x2):
y0 := prod(prod(x2, x0), x2inv):
y1 := prod(prod(x2, x1), x2inv):
y := prod(invers(y1), invers(y0)): outp(x0); outp(y0):
outp(x1); outp(y1); outp(x); outp(y)
```

The output is

```
[0, [11, 11, 11], [17, 17, 17]]
[0, [11, 11, 11], [44, 219, 177]]
[0, [23, 224, 138], [59, 136, 495]]
[0, [23, 224, 138], [33, 146, 501]]
[0, [28, 235, 129], [29, 211, 263]]
[0, [28, 235, 129], [58, 3, 445]]
```

The following lines carry out the conjugations:

```
a := op(2,x0):  b := op(2,x1):  c := 'mod'(a+b,2):
outp(x0); outp(conj(a,x0)); outp(conj(b,x0)); outp(conj(c,x0));
outp(y0); outp(conj(a,y0)); outp(conj(b,y0)); outp(conj(c,y0))
```

The output is (see also Appendix A(a) in the paper):

```
[0, [11, 11, 11], [17, 17, 17]]
[0, [11, 11, 11], [17, 17, 17]]
[0, [11, 11, 11], [31, 130, 117]]
[0, [11, 11, 11], [31, 130, 117]]
[0, [11, 11, 11], [44, 219, 177]]
[0, [11, 11, 11], [44, 219, 177]]
[0, [11, 11, 11], [34, 72, 213]]
[0, [11, 11, 11], [34, 72, 213]]
```

For powers of 2 we use the procedure `power2`, i.e.,

```
x0sq := power2(x0):  y0sq := power2(y0):
outp(x0sq); outp(conj(a,x0sq)); outp(conj(b,x0sq)); outp(conj(c,x0sq));
outp(y0sq); outp(conj(a,y0sq)); outp(conj(b,y0sq)); outp(conj(c,y0sq))
```

The output is (see also Appendix A(c) in the paper):

```
[1, [26, 26, 26], [0, 0, 0]]
[1, [26, 26, 26], [0, 0, 0]]
[1, [26, 26, 26], [0, 106, 247]]
[1, [26, 26, 26], [0, 106, 247]]
[1, [26, 26, 26], [0, 157, 106]]
[1, [26, 26, 26], [0, 157, 106]]
[1, [26, 26, 26], [0, 247, 157]]
[1, [26, 26, 26], [0, 247, 157]]
```

## 4. TREATMENT OF THE THIRD POWERS

For this aim, we use the following procedure, which calculates for given elements  $[0, U_1, U_2]$  and  $[1, V]$ , representing matrices  $M_0(U_1, U_2, \dots)$  and  $M_1(V, \dots)$ , their product  $[0, U_1, W]$ , representing a matrix  $M_0(U_1, W, \dots) = M_0(U_1, U_2, \dots)M_1(V, \dots)$ :

```
prod01 := proc(z,V)
local U1, U2, u11, u12, u13, u21, u22, u23, v1, v2, v3, res,
W, w1, w2, w3;
U1 := op(2,z); U2 := op(3,z);
u11 := extract(1,U1); u12 := extract(2,U1); u13 := extract(3,U1);
u21 := extract(1,U2); u22 := extract(2,U2); u23 := extract(3,U2);
v1 := extract(1,V); v2 := extract(2,V); v3 := extract(3,V);
w1 := 'mod'(u21+v1,2); w2 := 'mod'(u22+v2,2);
w3 := 'mod'(u23+v3,2);
W := comb(w1,w2,w3);
res := [0,U1,W]
end proc
```

The following lines generate then the third powers and their conjugates:

```
x0triple := prod01(x0,op(2,x0sq));
y0triple := prod01(y0,op(2,y0sq));
outp(x0triple); outp(conj(a,x0triple));
outp(conj(b,x0triple)); outp(conj(c,x0triple));
outp(y0triple); outp(conj(a,y0triple));
outp(conj(b,y0triple)); outp(conj(c,y0triple))
```

The output is (see also Appendix A(b) in the paper):

```
[0, [11, 11, 11], [11, 11, 11]]
[0, [11, 11, 11], [11, 11, 11]]
[0, [11, 11, 11], [5, 152, 111]]
[0, [11, 11, 11], [5, 152, 111]]
[0, [11, 11, 11], [54, 193, 171]]
[0, [11, 11, 11], [54, 193, 171]]
[0, [11, 11, 11], [56, 82, 207]]
[0, [11, 11, 11], [56, 82, 207]]
```

This finishes our explanations. We encourage the readers to check these and the other results in the paper using the above procedures or other procedures created by themselves...

(N. Barker and A. Vdovina) SCHOOL OF MATHEMATICS AND STATISTICS, NEWCASTLE UNIVERSITY, NEWCASTLE-UPON-TYNE, NE1 7RU, UK

*E-mail address:* `nathan.william.barker@gmail.com`

*E-mail address:* `alina.vdovina@ncl.ac.uk`

(N. Boston) DEPARTMENT OF MATHEMATICS, UNIVERSITY OF WISCONSIN, MADISON, WI 53706, USA

*E-mail address:* `boston@math.wisc.edu`

(N. Peyerimhoff) DEPARTMENT OF MATHEMATICAL SCIENCES, DURHAM UNIVERSITY, SCIENCE LABORATORIES SOUTH ROAD, DURHAM, DH1 3LE, UK

*E-mail address:* `norbert.peyerimhoff@durham.ac.uk`
